# Supplementary material for: AMuLeT: Automated Design-Time Testing of Secure Speculation Countermeasures
Source: arXiv:2503.00145 source file (2025-02-28)
Supplement: Supplementary file 1 [file 7.appendix.tex]

\rev{
\appendix 
\begin{appendices}
\section{Root-Causing Violations}
When \Gemfuzzer{} finds a violation, it outputs the program and inputs generating the violation
and the mismatching \utrace{s}. From this, we use a combination of scripts and manual analysis to determine
the root cause of the difference in \utrace{s}.

In this vein, we have developed a script which parses gem5's debug logs to provide a side-by-side
comparison of the speculative and non-speculative memory accesses performed by the program in the
two violating inputs, highlighting the ones that are different between them.
It also displays a full list of all squashes which occurred during the
program's execution, allowing us to quickly determine the cause of the speculation.
More sophisticated attacks such as those involving MSHR interference may still require manual
analysis of gem5's protocol trace.

Once we have determined the root cause of a violation, we either (a) develop a patch for the defense
to fix the vulnerability and re-run the fuzzer, or (b) write a script to filter out violations with the same root cause,
by searching for specific patterns in the \utrace{s} or gem5 debug log (e.g.\ for CleanupSpec, if the
difference between the \utrace{s} is two adjacent cache lines and there is a corresponding split request in the debug log,
then we mark it as a ``Split Requests Not Cleaned'' violation).
We repeat this process until the root causes of all remaining violations are established.
\end{appendices}

}
